# Supplementary material for: Simultaneous quantitative imaging of surface and magnetic forces
Source: arXiv:1303.2134 source file (2013-03-08)
Supplement: Supplementary file 1 [file Long_range_model_supplemental.pdf]

# Supplemental material: Simultaneous quantitative imaging of surface and magnetic forces

Daniel Forchheimer,[1] Daniel Platz,[1] Erik A. Tholén,[2] and David B. Haviland[1]

[1)] *Royal Institute of Technology, Stockholm*

[2)] *Intermodulation Products AB, Solna*

## I. COMPLETE PARAMETER IMAGES

Figure 1-4 shows the parameter images of all the free parameters from the two measurements (large oscillation amplitude and low oscillation amplitude). The position of the surface is the most sensitive parameter in the numerical fit. We have previously found that it is advantageous to parametrize the position of the surface with respect to the lowest turning point of the cantilever, rather than the equilibrium point. Thus in the fit for the large oscillation amplitude measurement we used $z_{pen} = d_{turn} - d_s$ as the free parameter rather than $d_s$ where $z_{pen}$ is the penetration depth into the surface, $d_s$ the position of the surface with respect to tip deflection and $d_{turn}$ the position of the lowest deflection turning point. For the non-contact measurement the parameter $z_{dist} = -(d_s - d_{turn})$ was used to pin the position of the surface below the lowest deflection.

## II. FORCE VOLUME SLICE MOVIES

Movies sweeping through the force volume are available online. *xy_force.mp4* shows the force in the $x - y$ plane for the large oscillation amplitude. *xz_force.mp4* shows the force in the $x - z$ plane for the large oscillation amplidute. *xz_force_noncontact.mp4* shows the force in the $x - z$ plane for the low oscillation amplitude.

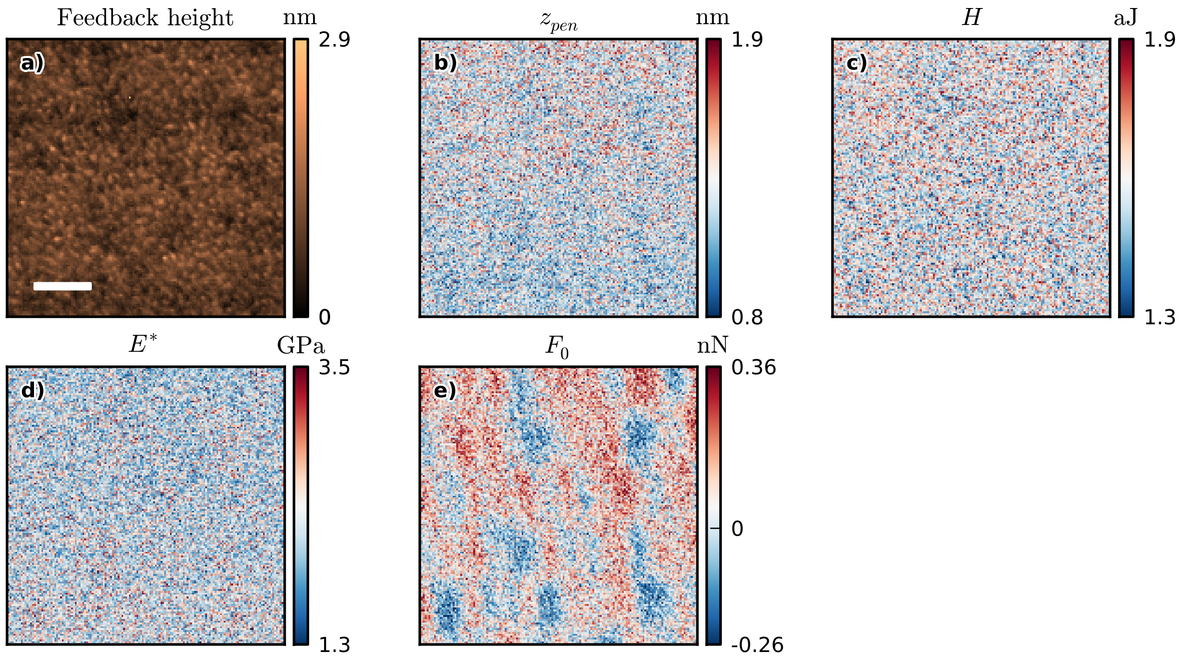


FIG. 1. Large oscillation amplitude. No smoothing

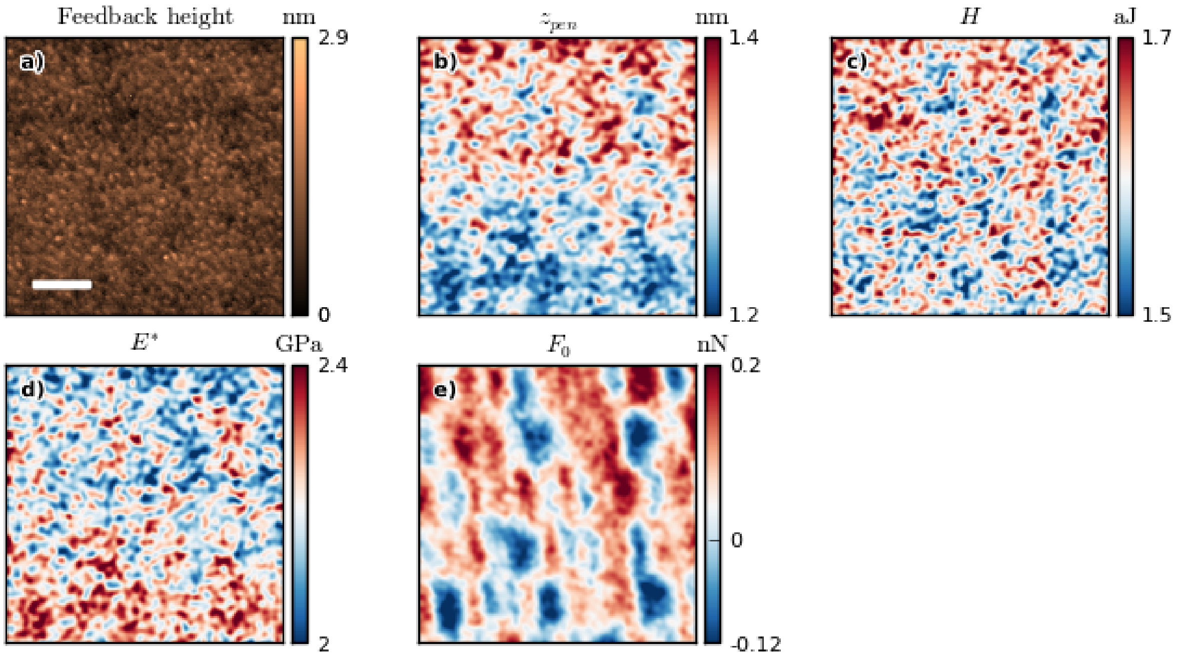


FIG. 2. Large oscillation amplitude. Smoothed with $\sigma = 10$ nm

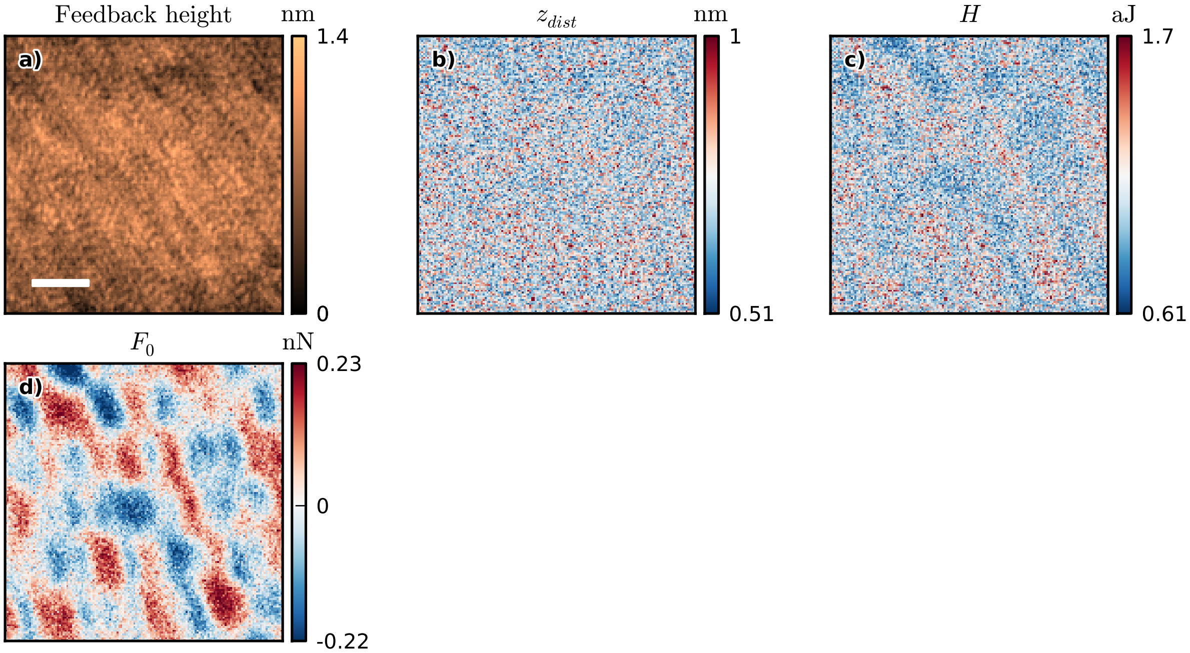


FIG. 3. Low oscillation amplitude. No smoothing

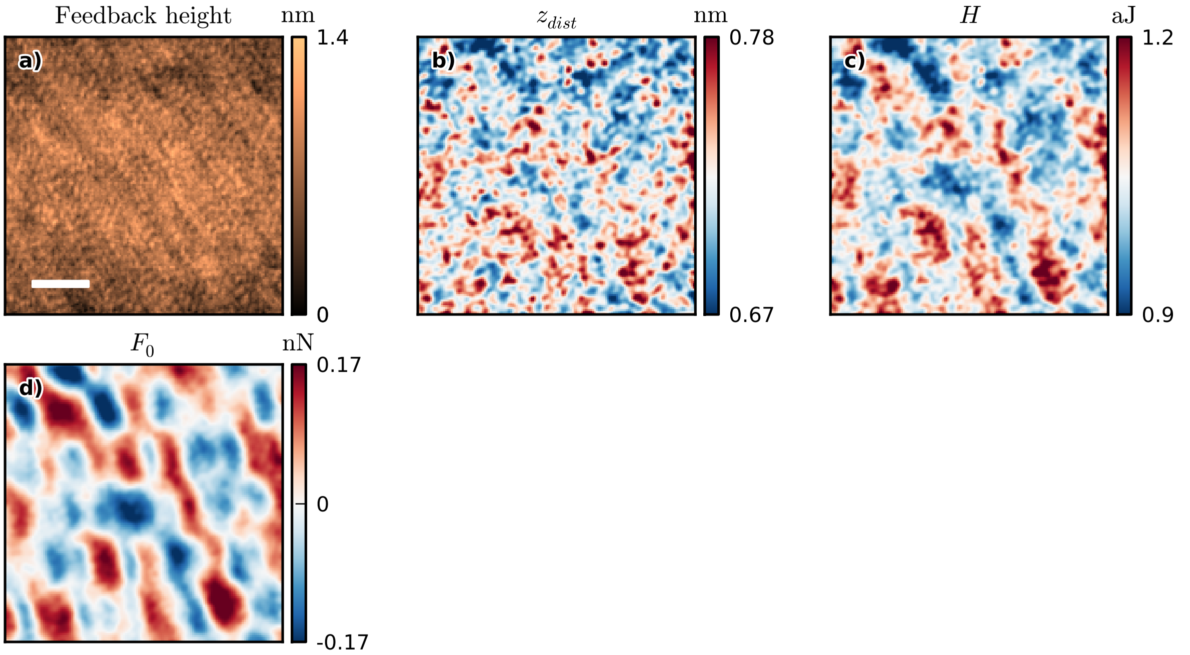


FIG. 4. Low oscillation amplitude. Smoothed with $\sigma = 10$ nm
